# Supplementary material for: HDR-Plenoxels: Self-Calibrating High Dynamic Range Radiance Fields
Source: arXiv:2208.06787 source file (2022-11-18)
Supplement: Supplementary file 1 [file qual_baseline.tex]

\begin{figure}[t]
\setlength{\abovecaptionskip}{0mm} 
    \centering
    \includegraphics[width=1\linewidth]{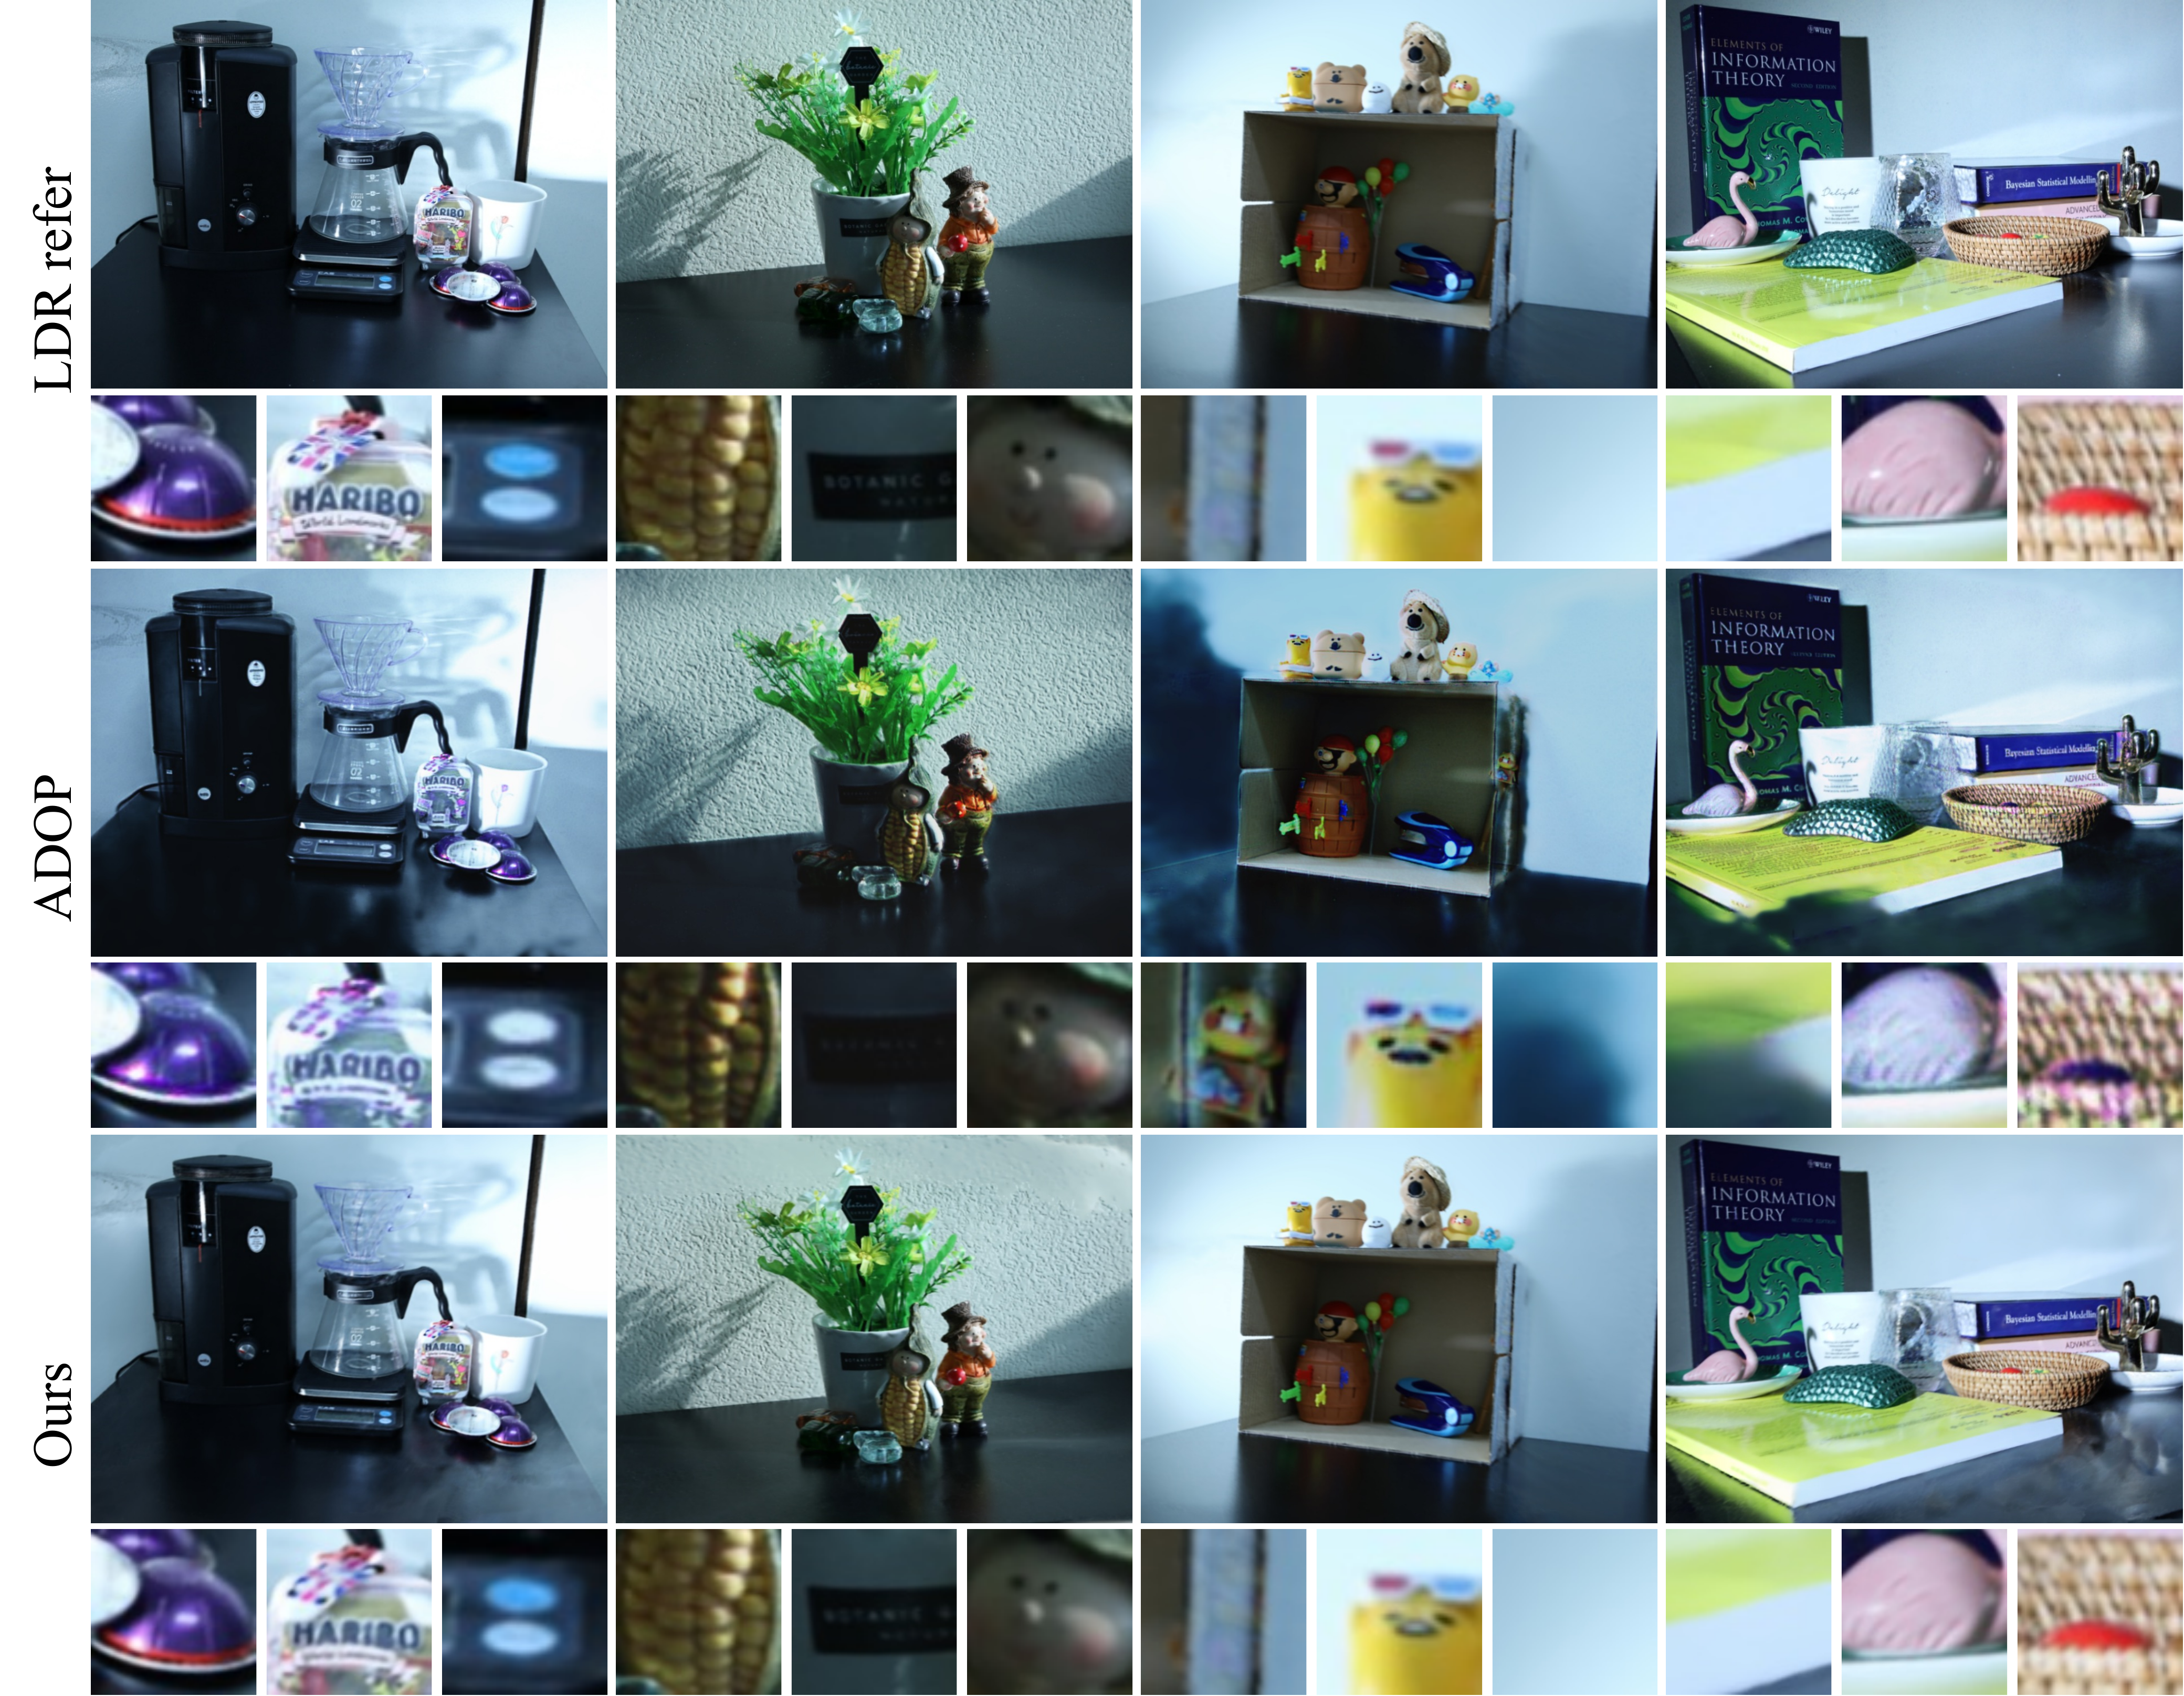}
    % \vspace{-7mm}
    \caption{\textbf{Comparisons of qualitative results to baseline.}
    The first row represents the LDR reference image, which is used at training.
    All experiments are trained with varying conditioned data and rendered with tone mapping stage.
    Our results represent fine-grained rendering results compared to the ADOP baseline.
    Especially, ours shows satisfying color representations compared to ADOP.
    }
    \label{sup_fig:baseline}
    % \vspace{-3mm}
\end{figure}
