# Supplementary material for: HDR-Plenoxels: Self-Calibrating High Dynamic Range Radiance Fields
Source: arXiv:2208.06787 source file (2022-11-18)
Supplement: Supplementary file 2 [file qual_crf_rgb.tex]

\begin{figure}[t]
    \centering
    \includegraphics[width=1\linewidth]{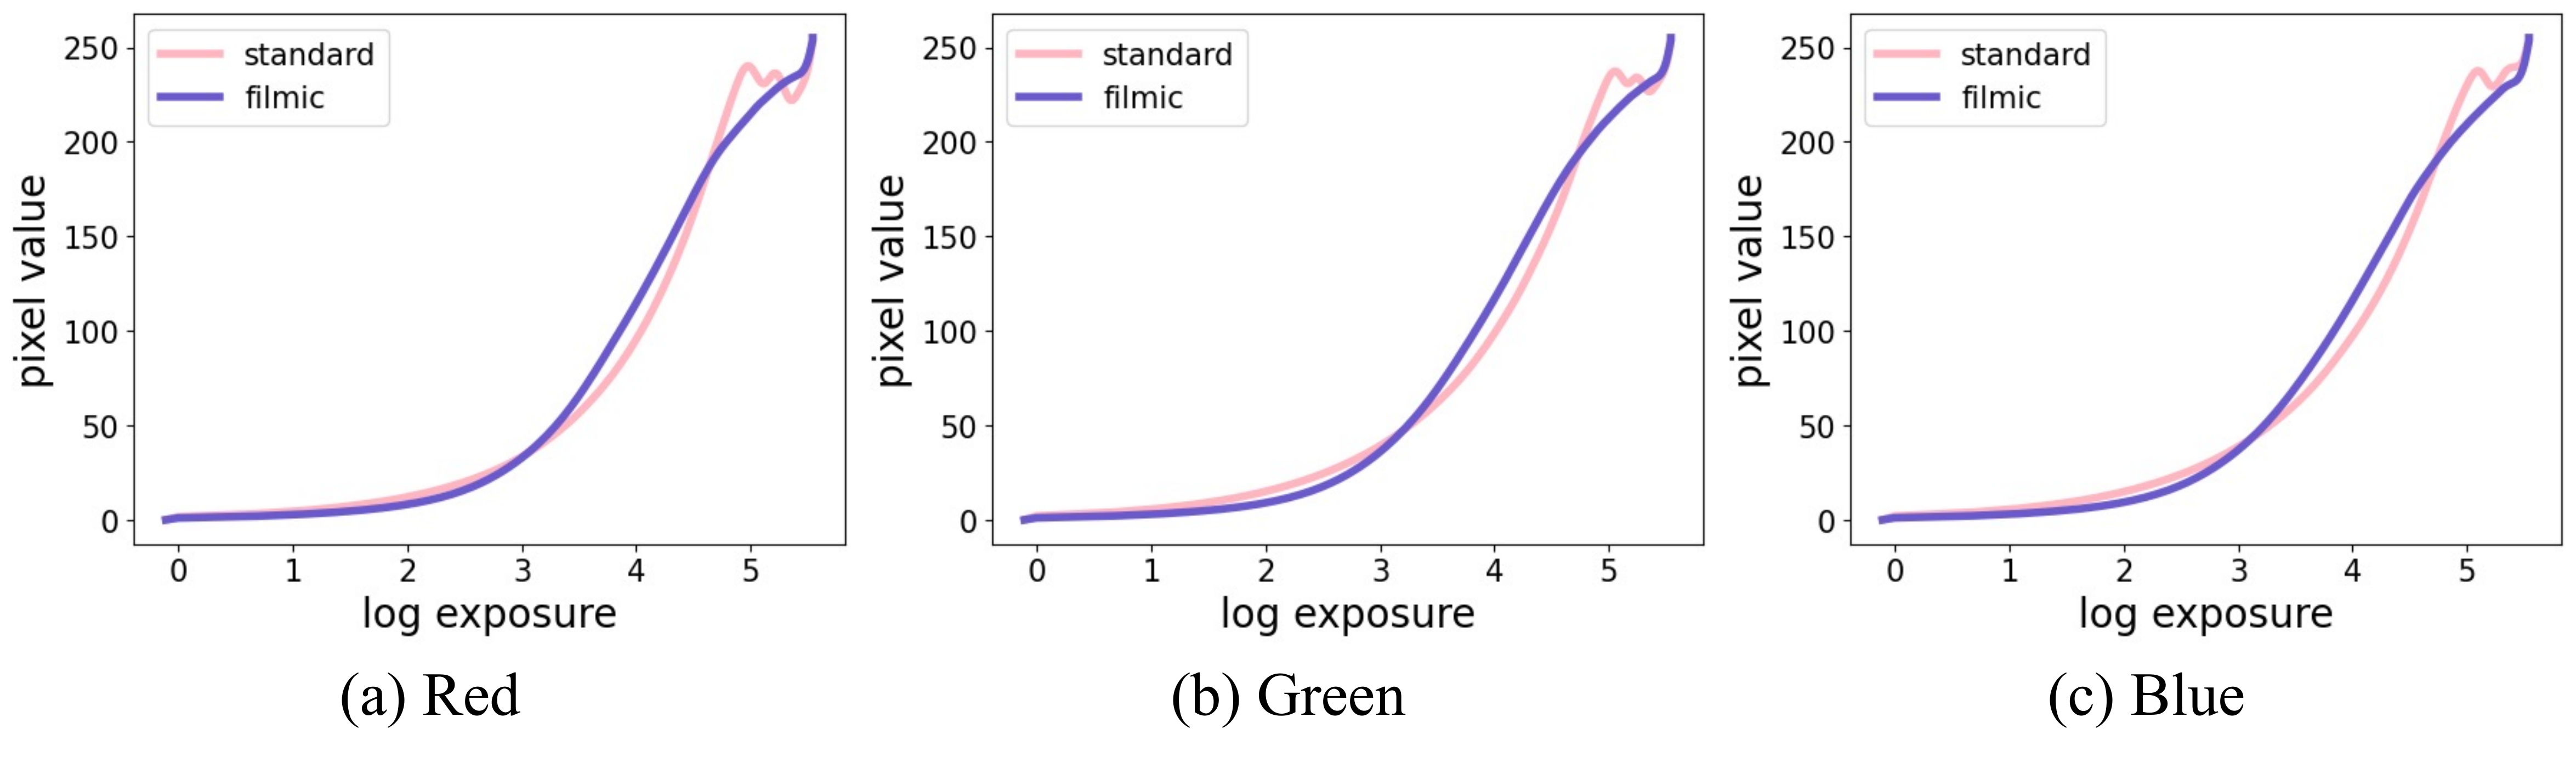}
    % \vspace{-7mm}
    \caption{\textbf{CRF according to color channels.}
    There are comparisons of CRF function at each color channel between standard and filmic transforms.}
    \label{sup_fig:crf_rgb}
    % \vspace{-5mm}
\end{figure}
