# Supplementary material for: HDR-Plenoxels: Self-Calibrating High Dynamic Range Radiance Fields
Source: arXiv:2208.06787 source file (2022-11-18)
Supplement: Supplementary file 3 [file qual_denoise.tex]

\begin{wrapfigure}{r}{0.40\linewidth}
  \setlength{\abovecaptionskip}{-1mm}
  \centering
  \includegraphics[width=1\linewidth]{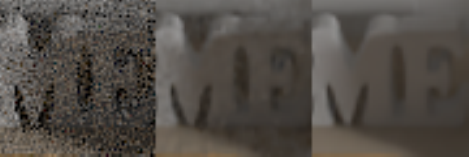}
  \caption{\textbf{Denoising effect of HDR-Plenoxels.}}
    % Images show input kitchen data with shot noise (left) and qualitative result of our models trained on images with (middle) or without shot noise (right). Our model show denoising effects to some extent.
    % }
    \label{sup_fig:qual_denoise}
\end{wrapfigure}
