# Supplementary material for: HDR-Plenoxels: Self-Calibrating High Dynamic Range Radiance Fields
Source: arXiv:2208.06787 source file (2022-11-18)
Supplement: Supplementary file 6 [file quan_extreme.tex]

\begin{table}
\setlength{\abovecaptionskip}{2mm}
\setlength{\belowcaptionskip}{1mm}
    \centering
    \small
    \caption{\textbf{PSNR on extreme conditions.}}
    % We consider replacing the averaging in $\gs$ with either max-pooling or the class token. We show ImageNet-1K \ug{top-1 accuracy} on the validation set.}
    \label{table:hard}
    \resizebox{0.5\linewidth}{!}{
    \begin{tabular}{c CCCC}
         \toprule
          Exposure & $\pm$3EV & $\pm$4EV & $\pm$5EV & $\pm$6EV\\
         \midrule
         PSNR & $\ourpsnr$ & 30.30 & 29.10 & 28.48\\
         \bottomrule
    \label{sup_table:quan_extreme}
    \end{tabular}}    
\end{table}
