# Supplementary material for: HDR-Plenoxels: Self-Calibrating High Dynamic Range Radiance Fields
Source: arXiv:2208.06787 source file (2022-11-18)
Supplement: Supplementary file 7 [file D.3.HDR_metric.tex]

\subsection{Comparison of reconstructed HDR to HDR GT}
% We report the updated version of the HDR-VDP metric~\cite{HDR-VDP-2}, which ranges in $[0,10]$, and follow the normalization~\cite{liu_single-image_2020} to deal with scale-ambiguity with our HDR results.
% Ours achieves 4.29$\pm$1.81 while ADOP achieves 3.97$\pm$1.72.
% Ours learns high-quality HDR results compared to ADOP.
% Our model can also produce more accurate results in HDR image rendering compared to ADOP.
To quantify the exactness of the HDR rendering, we adopt the HDR-VDP metric~\cite{HDR-VDP-2}.
We employ an updated version of HDR-VDP, which ranges in $[0,10]$ and follow the normalization~\cite{liu_single-image_2020} to deal with scale-ambiguity with our HDR results.
We measured HDR-VDP on all of our synthetic data.
Ours achieves 4.29$\pm$1.81 while ADOP achieves 3.97$\pm$1.72.
HDR-Plenoxels can learn precise results not only in LDR but also in HDR rendering.
